# Supplementary material for: INT2.1: Towards Fine-Tunable Quantized Large Language Models with Error Correction through Low-Rank Adaptation
Source: arXiv:2306.08162 source file (2023-06-13)
Supplement: Supplementary file 1 [file Appendix.tex]

\documentclass{article}

% if you need to pass options to natbib, use, e.g.:
%     \PassOptionsToPackage{numbers, compress}{natbib}
% before loading neurips_2023

% ready for submission
\usepackage{neurips_2023}

% to compile a preprint version, e.g., for submission to arXiv, add the
% [preprint] option:
%     \usepackage[preprint]{neurips_2023}

% to compile a camera-ready version, add the [final] option, e.g.:
%     \usepackage[final]{neurips_2023}

% to avoid loading the natbib package, add option nonatbib:
%    \usepackage[nonatbib]{neurips_2023}

\usepackage[utf8]{inputenc} % allow utf-8 input
\usepackage[T1]{fontenc}    % use 8-bit T1 fonts
\usepackage{hyperref}       % hyperlinks
\usepackage{url}            % simple URL typesetting
\usepackage{booktabs}       % professional-quality tables
\usepackage{amsfonts}       % blackboard math symbols
\usepackage{nicefrac}       % compact symbols for 1/2, etc.
\usepackage{microtype}      % microtypography
\usepackage{xcolor}         % colors
\usepackage{amsmath}
\usepackage{amssymb}
\usepackage{multirow}
\usepackage{graphicx}
\usepackage{caption} 
\captionsetup[table]{skip=5pt}
\captionsetup[figure]{skip=10pt}

\begin{document}
\appendix
\input{Appendix/AppendixA}
\input{Appendix/AppendixB}
\input{Appendix/AppendixC}
\input{Appendix/AppendixD}
\end{document}
